# Supplementary material for: Simple yet Effective Node Property Prediction on Edge Streams under Distribution Shifts
Source: arXiv:2504.00328 source file (2025-04-01)
Supplement: Supplementary file 1 [file 99_appendix_additional_discussion.tex]

\blue{\section{Appendix: Additional Discussion and Analysis}}
\label{sec:app:add_discuss}
\blue{\subsection{Discussion on Normal Pattern Assumptions}}
\label{sec:disucussion_pattern}
\blue{
As mentioned in Section~\ref{sec:method}, the intuition of our normal pattern assumptions is that normal nodes engage in repetitive and sustained interaction with similar neighbors over time.
To support this, we aim to explore social and psychological research to explain the underlying reasons.
In \citep{goerzen2007alliance}, the authors explain that repeated interactions raise trust between members, reducing the need for contractual safeguards in subsequent alliances. Therefore, the economic logic of repeated interactions with similar neighbors is the cost-saving benefits of trust. 
\citep{roberts2009exploring} mentions that there are constraints on the number of relationships the ego can maintain. These constraints are expected to be cognitive (the size of an individual's support clique is correlated with the number of levels of intentionality that an individual can process) and time budgeting.
Additionally, \citep{garbarino1999different} explains that repeated and sustained interactions are expected as evidence of a relationship.
As a result, we can infer that normal nodes establish relationships with a limited number of neighbors and consistently engage in repetitive interactions with them, which supports our normal pattern assumptions.
}

\blue{\subsection{Training Complexity Analysis}}
\label{sec:disucussion_training_complex}
\blue{
We roughly analyze the training time complexity of \method. 
Specifically, we examine the forward cost of (a) temporal contrast loss and (b) memory generation loss for a temporal edge $(v_{i},v_{j},t)$ in the training set. 
}

\blue{
\smallsection{Temporal Contrast Loss}
Given a training edge, \method updates the memory vector of each node in the edge using GRU. 
The total time complexity is dominated by that of GRU, which is $\calO({d_{s}}^{2}+d_{s}d_{m})$~\citep{rotman2021shuffling}, where $d_{s}$ and $d_{m}$ indicate the dimensions of memory vectors and messages respectively. 
Then, SLADE computes the similarities (a) between the current memory and previous memory and (b) between current memory and memories of negative samples for each node in the training edge. 
It takes $\calO(\mathcal{V}_{n}{d_{s}}^{2})$, where $\mathcal{V}_{n}$ is the number of negative samples.
}

\blue{
\smallsection{Memory Generation Loss}
Given a training edge, \method generates memory vectors for nodes in the training edge using TGAT with the time complexity of $\calO(k{d_{s}}^{2})$~\citep{zheng2023temporal}, as mentioned in Section 5.2.
Then, \method computes the similarities (a) between generated memory and current memory vectors and (b) between generated memory and memories of negative samples for each node in the training set, taking $\calO(\mathcal{V}_{n}{d_{s}}^{2})$ time.
}

\blue{
As a result, the time complexity of computing both losses for a training edge is $\mathcal{O}((k+\mathcal{V}_{n}){d_{s}}^{2}+d_{s}d_{m})$.
In the worst case, using $\mathcal{V}(t^{+})$ as negative samples can result in the time complexity of $\mathcal{O}((k+\mathcal{V}_{t}){d_{s}}^{2}+d_{s}d_{m})$, where $\mathcal{V}_{t}$ is the number of nodes in the training set.
Therefore, with our current negative sampling method, the training time increases as the number of nodes in the training set increases.
In our experiments in Appendix D.3, we observe that the number of nodes in the training set does not significantly affect training time on the Reddit dataset.
However, as shown in Appendix D.9, the number of nodes in the training set affects training scalability on large-scale datasets.
It is necessary to explore methods to limit the number of negative samples effectively.
}
