# Supplementary material for: Simple yet Effective Node Property Prediction on Edge Streams under Distribution Shifts
Source: arXiv:2504.00328 source file (2025-04-01)
Supplement: Supplementary file 2 [file 99_appendix_baseline.tex]

\section{Appendix: Baseline Method Details}
\label{sec:app:baseline}
Among the four experiments mentioned earlier, the last type analysis experiment utilizes only unsupervised baselines. we provide individual baselines for the main experiments (RQ1, RQ2, RQ3) and the type analysis experiment (RQ4).

\subsection{Details of Baselines in Main Experiments}
\label{sec:app:base:baseline_main}
We compare the performances of our proposed method and the nine baseline methods in detecting dynamic anomalies in edge streams.
The used baseline methods can be categorized as below:
\begin{itemize}[leftmargin=*]
    \item \textbf{Rule-based:} \SedanSpot~\citep{eswaran2018sedanspot}, \MIDAS~\citep{bhatia2020midas}, \FFADE~\citep{chang2021f}, and \Anoedgel \citep{bhatia2021sketch}
    \item \textbf{Neural network-based:} \JODIE~\citep{kumar2019predicting}, \Dyrep~\citep{trivedi2019dyrep}, \TGAT~\citep{xu2020inductive},  \TGN~\citep{tgn_icml_grl2020}, and \SAD~\citep{tian2023sad}
\end{itemize}
%Note that all used methods are capable of applying to CTDG.

%In rule-based approaches, although the training phase and feature information is not required, some level of hyperparameter tuning is necessary to achieve sufficient performance.
For rule-based approaches, although the training phase is not necessary, some level of hyperparameter tuning can greatly increase the performance of them in our task.
For a fair comparison, for each dataset, the optimal hyperparameter setting of each rule-based method is determined using the validation set. 
%Then for each dataset, we evaluate the corresponding model in a test set with the selected hyperparameter setting.
The selected hyperparameter setting is used to evaluate the corresponding model in the test set.
There are several details regarding some of the used baseline methods:
\begin{itemize}
    \item \textbf{Anoedge-l:} \citet{bhatia2021sketch} propose several versions of Anoedge. Among them, we adopt \textbf{Anoedge-l} as our baseline method since it exhibits the best performance among them in our task.
    \item \textbf{MIDAS-R:} \citet{bhatia2020midas} propose several versions of MIDAS. 
    Among them, we adopt \textbf{MIDAS-R} as our baseline method since it outperforms the others in our preliminary study.
    \item \textbf{F-FADE:} This method processes a stream every minute, while interactions in the used datasets occur at a much dense time interval (i.e., tens of interactions on original datasets occur within a minute).
    Due to this characteristic, F-FADE always underperforms all other used methods, specifically, cannot capture any anomalies. 
    For F-FADE, we modify each dataset by adjusting the time units to large intervals. 
\end{itemize}
%Subsequently, the model's performance is evaluated on a test set.
%Specifically, we choose MIDAS-R over the standard MIDAS model as we expect that MIDAS-R would exhibit better performance in capturing dynamic anomalies.
%Specifically, we choose MIDAS-R over the standard MIDAS model as we expect that MIDAS-R would exhibit better performance in capturing dynamic anomalies.
%\citep{bhatia2021sketch} propose two methods for anomalous edge detection, Anoedge-l and Anoedge-g. We select Anoedge-l due to its better performance on our task.
%\red{In the case of F-FADE, this method requires multiple occurrences of the same edge within the same timestamp. 
%However, our datasets granularity have a more refined time interval, which makes it challenging to apply F-FADE directly. 
%Therefore, we have to modify the dataset by adjusting the time units to large intervals for applying the F-FADE model.}

%In neural network-based approaches, the training process involves using the training set for model training and the validation set for finding the optimal hyperparameters. 
%Fortunately, these baselines have official hyperparameter settings for implementations in \citep{xu2020inductive,tgn_icml_grl2020,tian2023sad}. 
%Therefore, we utilize the reported hyperparameter settings for each baseline and additional hyperparameter settings derived through validation.

%When conducting testing with the optimal hyperparameter settings, two strategies are employed. 
In neural network-based methods, except for our proposed method, after selecting the hyperparameter settings based on its validation set, there are two strategies for utilizing a given dataset (train set and validation set) for training the final representation model with the selected hyperparameter settings:

\begin{itemize}[leftmargin=*]
    \item \textbf{S1. Using Both:} This indicates using both train and validation sets to train the final representation model with the selected hyperparameter settings. 
    In this case, the model may utilize more information during training, while the model gets vulnerable to the overfitting issue.
        \item \textbf{S2. Training Set Only:} This indicates using only the train set to train the final representation model with the selected hyperparameter settings. 
    In this case, the model utilizes the validation set only for early stopping, but we do not fully utilize the given dataset during training.
    
\end{itemize}
For each model, except for SAD (since the method inherently utilizes a validation dataset during model training), we utilize both strategies and report the higher test set evaluation performance between them.

%The first involves merging the training and validation sets for combined training and then evaluating the model's performance on the test set.
%The second strategy perform model training on the training set and using the validation set for model selection and then evaluating the selected model's performance for testing.
%Both of these strategies have their own advantages and disadvantages (Including the validation set in the training process often leads to improved overall performance, On the other hand, leveraging the validation set for model selection often is more robust to the overfitting), we try both approaches and report best performance between them.
%With one exception, SAD utilize the validation set for model selection as default within the model itself.

%To measure the quality of the inductive biases inherent in the encoder model, we also consider \RandomInit~\citep{velivckovic2018deep,thakoor2021large}, an encoder with the same architecture as \method but with randomly initialized parameters, as a baseline.
%Since the methods working on graphs can not be directly applied to hypergraphs, we use them after transforming hypergraphs to graphs via clique expansion.
%In the case of \HHGR, it is originally designed for group recommendations with supervisory signals, and therefore it is not directly applicable to node classification tasks.
%Thus we slightly modified the algorithm so that it uses only its self-supervised loss.
%For all the baseline approaches, we report their performance using their official implementations.

\subsection{Details of Baselines in Type Analysis Experiments}
\label{sec:app:base:baseline_real}
We compare the performances of our proposed method and four unsupervised baseline methods in type analysis. The unsupervised baseline methods are as follows: {\SedanSpot~\citep{eswaran2018sedanspot}, \MIDAS~\citep{bhatia2020midas}, \FFADE~\citep{chang2021f}, and \Anoedgel~\citep{bhatia2021sketch}.}
% \begin{itemize}
%     \item \textbf{Rule-based:} \SedanSpot~\citep{eswaran2018sedanspot}, \MIDAS~\citep{bhatia2020midas}, \FFADE~\citep{chang2021f}, and \Anoedgel~\citep{bhatia2021sketch}
% \end{itemize}
In the Synthetic-hijack and Synthetic-New datasets, anomalies exist only in the test set, making it impossible to conduct a validation.
Thus, for each model, we utilize the hyperparameter combinations the respective paper has reported.
%Consequently, we utilize the reported hyperparameter settings in previous studies.
In cases where baseline settings in the previous work vary across datasets, we use the combination that has shown good performance in our main experiments (Section~\ref{sec:exp:classification}).
