# Supplementary material for: Simple yet Effective Node Property Prediction on Edge Streams under Distribution Shifts
Source: arXiv:2504.00328 source file (2025-04-01)
Supplement: Supplementary file 3 [file 99_appendix_dataset.tex]

\section{APPENDIX: Dataset Details}
\label{sec:app:dataset}

\subsection{Real-world Datasets}
\label{sec:app:real_dataset}
We use 7 real-world datasets for a node property prediction task;
three datasets (Wikipedia, Reddit, and MOOC~\cite{kumar2019predicting})~\footnote{http://snap.stanford.edu/jodie/\#datasets} for dynamic anomaly detection and two datasets (Email-EU~\cite{paranjape2017motifs}~\footnote{https://snap.stanford.edu/data}, GDELT~\cite{zhou2022tgl}~\footnote{https://s3.us-west-2.amazonaws.com/dgl-data/dataset/tgl/GDELT}) for dynamic node classification, and two datasets (TGBN-trade and TGBN-genre~\cite{huang2024temporal})~\footnote{https://tgb.complexdatalab.com/docs/nodeprop/} for node affinity prediction.
Basic descriptive statistics of each dataset are provided in Table~\ref{tab:dataset} of Section~\ref{sec:exp:details}.
Below, we provide a detailed description of each dataset.

\smallsection{Datasets for Dynamic Anomaly Detection}
The Wikipedia dataset records edits made by users on Wikipedia pages.
The Reddit dataset consists of posts made by users on subreddits. 
In the Wikipedia and Reddit datasets, if an administrator bans a user at a specific time, the user is assigned an abnormal property after that time; otherwise, it has a normal property. 
The MOOC dataset consists of user activities on MOOC online course platforms.
In the MOOC dataset, if a user drops the course at a particular time point, it is marked with an abnormal property after that time point; otherwise, it has a normal property. 

\smallsection{Datasets for Dynamic Node Classification}
The Email-EU dataset consists of emails between users in a European research institution.
The property of a user at a specific time indicates the user's department ID at the institute, which remains constant over time in this dataset.
The GDELT dataset is an event network that records events worldwide between actors from GDELT 2.0 ~\cite{leetaru2013gdelt}. Following the ~\cite{cong2022we}, the GDELT dataset is sub-sampled for single-machine training.
The location (country) of an actor at a specific time is considered a property, which is dynamic over time.
Unlike other datasets, the GDELT dataset has node features that are multi-hot vectors representing the CAMEO codes attached to the actors.

\smallsection{Datasets for Node Affinity Prediction}
The TGBN-trade dataset records international agriculture trading between nations of the UN. Each node is a nation, and the edge weight represents the sum of the agricultural product value traded between the two nations. 
The property of a nation is the proportion of agricultural trade values to other nations during the next year.
The TGBN-genre is a weighted interaction network between users and the music genres of songs they listen to. 
The edge weights represent the percentage of a song's association with a particular genre.
The property of a user is the user's preference of music genres over the next week.
In such cases, previous studies have incorporated edge weight as an edge feature because the models can not explicitly handle edge weight. 
Consequently, edge weight is utilized as an edge feature for existing models in our experiments.
Note that these property labels from all datasets are inherently given in the original datasets.
%In Wikipedia and Reddit datasets, which are social networks between users, a user's property at time $t$ indicates the user's state at time $t$. 
%Specifically, if a user is banned by administrators at time $t$, the property label of the user at time $t$ is marked as one.
%In the MOOC dataset, which consists of user activities on the online platform, if a user drops the course at time $t$, the property label of the user at time $t$ is marked as one.
%Otherwise, the user has a property label of zero.
%In addition, each edge has associated edge features in these datasets, but no specific edge weight is provided, so all edges are assigned a weight of one.

\subsection{Details of Synthetic Datasets}

In this section, we provide more details of synthetic datasets.
%We create synthetic datasets to evaluate the robustness of \method and other baselines under artificial distribution shifts.
The synthetic dataset consists of 1,000 nodes, each belonging to one of 10 classes, which are static over time, with 100 nodes per class. ~\footnote{Each node belongs to a class determined by the quotient obtained by dividing its node ID by 100.}
A total of 20,000 temporal edges occur over 0 to 1,000,000 seconds, and the goal is to predict the class of each source node as the node property. 
We utilize the same chronological 10/10/80$\%$ split for training, validation, and test sets. 
In this case, labels of source nodes within temporal edges within the training set can be utilized for training.

As mentioned in Section V, to induce distribution shifts, we manipulate the frequency of node appearances between the training and test sets according to the class using a shift intensity factor $p$, which ranges from 50 to 100.
Specifically, we first sample class-known node sets for each class, consisting of nodes that can appear as source nodes in the training set. we sample $p$ nodes as class-known nodes per class for group 1 classes and sample (100-$p$) nodes as class-known nodes per class for group 2 classes.
The nodes that are not sampled are assigned to the class-unknown sets for each class.

When generating temporal edges in the training set, source nodes are selected from the class-known node sets of group 1 classes with a probability of $p\%$ or from the class-known node sets of group 2 classes with a probability of $(100-p)\%$.
The destination nodes are selected from the same class as the source nodes with a probability of 90\%, or they are randomly selected with a probability of 10\%.

In contrast, temporal edges in the validation and test set are generated in reverse.
When generating temporal edges in the test set, source nodes are selected from the class-unknown node sets of group 1 classes with a probability of $(100-p)\%$ or from the class-unknown node sets of group 2 classes with a probability of $p\%$.
The selection process for destination nodes is the same as for the training set.
The timestamps are uniformly distributed across the entire range of temporal edges for the training, validation, and test sets, and selected randomly within their respective ranges.

\subsection{Distribution Shifts Analysis}
\label{dist_shift_all_data}
\smallsection{Distribution Shifts in Real-world Datasets}
In this section, we aim to analyze distribution shifts across 6 real-world datasets (except the Reddit dataset), similar to the analysis conducted in Section ~\ref{sec:intro}.
\begin{itemize}[leftmargin=*]
    \item \textbf{Positional Distribution Shifts:} To analyze positional shifts in real-world datasets, we first divide the nodes into 20 groups~\footnote{In TGBN-trade, we utilize the 10 groups due to the small number of nodes.} based on their appearance time in the CTDG. Node embeddings are then generated by applying node2vec to the entire graph. Finally, we visualize the average embedding of each group using a t-SNE plot.
    As shown in Figure~\ref{fig:pos_shift_example}, we can observe that the distribution of embeddings representing the positions of nodes appearing over time varies in most datasets. 
    %we can observe the positional distribution shifts in real-world network datasets. Especially as the available training range decreases, the proportion of nodes visible to the model further declines, increasing the impact of the positional distribution shift.
    \item \textbf{Structural Distribution Shifts:} According to Figure~\ref{fig:str_shift_example}, we can observe that the average degree of nodes increases over time across all datasets, indicating a structural distribution shift.
    In the case of the TGBN dataset, the average node degree is quite large over time, which means that if the number of sampled neighbors is too small, it may not adequately capture these structural shifts.
    \item \textbf{Property Distribution Shifts:} As shown in Figure~\ref{fig:property_shift_example}, the occurrence rate of node properties varies over time, showing a property distribution shift.
    Therefore, to effectively address these shifts, it is essential to identify node characteristics that have a stable relationship with node properties over time.
\end{itemize}

\smallsection{Distribution Shifts in Synthetic Datasets}
In this section, we aim to analyze distribution shifts in the synthetic datasets (Synthetic-50, Synthetic-70, and Synthetic-90) with the artificial positional distribution shifts.
We adopt a similar approach for real-world networks to analyze positional shifts in the synthetic datasets without averaging the embeddings.
As shown in Figure~\ref{fig:synthetic_shift_analysis}, We observe that positional shifts are more distinct in the datasets with higher shift intensity factor $p$.

\input{tables/all_dataset_positional_shift}

\input{tables/all_dataset_structural_shift}
\input{tables/all_dataset_property_shift}

\begin{figure}[t]
    \centering
    \includegraphics[width=0.48\textwidth]
    {figs/synthetic_pos_shift_v3.png}
    \caption{ \label{fig:synthetic_shift_analysis}
        positional distribution shifts analysis plot in Synthetic-50, 70, and 90.  Nodes are grouped based on their appearance time, and the node embeddings generated by node2vec using the entire graph. 
        These node embeddings are visualized using t-SNE. Positional shifts are more noticeable in datasets with a higher shift intensity factor.
    }
\end{figure}
