# Supplementary material for: Simple yet Effective Node Property Prediction on Edge Streams under Distribution Shifts
Source: arXiv:2504.00328 source file (2025-04-01)
Supplement: Supplementary file 4 [file 99_appendix_exp.tex]

\section{Appendix: Additional Experiments}
\label{sec:app:exp}

\input{tables/accuracy_SF_switch}
 \subsection{Performance of Baselines using Selected Augmentation Node Features}
\label{sec:app:exp:baseline_SF}
In this subsection, we evaluate each model with the selected augmented node features regarding  RQ1 on four real-world datasets (Wiki, Reddit, Email-EU, and TGBN-trade). 
All TGNN baselines use the selected augmented node feature with minimal empirical risk for each dataset, according to the results in Table~\ref{tab:ablation_selection}.

As shown in Table~\ref{tab:SF_performance}, utilizing the selected augmented node feature improves model performance in many cases.
Specifically, for the Email-EU dataset, all baselines with selected augmented node features exhibit significant performance improvements.
In the cases where the selected augmented node features are utilized, \method outperforms other complex TGNN models across four datasets. 
This result demonstrates that a simple model with proper node features has advantages in predicting node properties under distribution shifts, offering better performance and generalization ability.

\input{tables/training_time_analysis}

\subsection{Model Training Speed}\label{sec:app:exp:training}
In this subsection, we analyze the training time of \method.
We compare the empirical training time of \method against that of other TGNN baselines.
In this case, we run each model for 10 epochs with the same batch size of 600 and report the average training time.
According to the results in Figure~\ref{fig:training_speed}, SPLASH demonstrates the best trade-off between training speed and performance compared to other models on the Reddit dataset.
%As shown in the right plot of Figure~\ref{fig:trianing_time_analysis}, in terms of the empirical training speed, \method is competitive compared to other methods.
Specifically, \method is 64.90$\times$ faster than the second-best performing baseline, DyGFormer+R in the training.
\method significantly outperforms JODIE, the fastest model, with a 33.24$\%$ performance gain.
