# Supplementary material for: Simple yet Effective Node Property Prediction on Edge Streams under Distribution Shifts
Source: arXiv:2504.00328 source file (2025-04-01)
Supplement: Supplementary file 5 [file 99_appendix_implementation.tex]

\input{tables/HP_setting_switch}
\section{Appendix: Implementation Details}
\label{sec:app:impl}

%In this section, we provide some details about our implementation, including the experiment environment and hyperparameters.

\subsection{Experiments Environment}
\label{sec:app:impl:infra}
We conduct all experiments with NVIDIA RTX 3090 Ti GPUs (24GB VRAM), 256GB of RAM, and two Intel Xeon Silver 4210R Processors.

\subsection{Details of Evaluation Metrics and Baselines}
\label{sec:app:impl:baseline_param}

\smallsection{Details of Evaluation Metric}
We introduce the evaluation metrics for each subtask in this section as follows:
\begin{itemize}[leftmargin=*]
    \item \textbf{AUC:} In anomaly detection, AUC is a performance metric commonly used to evaluate the performance of a model.
    It refers to the area under the Reciever Operating Characteristic (ROC) curve, which plots the true positive rate (TPR) against the false positive rate (FAR) at various classification thresholds.
    A higher AUC indicates that the model effectively detects anomalies across most thresholds, reflecting strong performance.
    \item \textbf{F1 Score:} In node classification, F1 Score is a general performance measure to evaluate a model's performance by balancing precision and recall.
    A high F1 Score indicates overall strong performance in correctly identifying and classifying nodes within the graphs.
    \item \textbf{NDCG@k:} In the recommender system, NDCG@k is a commonly used metric to evaluate the quality of ranking models. 
    It refers to the Normalized Discounted Cumulative Gain metric that considers the relative order of elements.    It measures how closely the top-k predicted items align with users' actual item preference rankings.
    A high NDCG@k indicates that the predictions closely match the users' actual item preference rankings, reflecting strong recommendation performance.
\end{itemize}

\smallsection{Details of Baselines}
As mentioned in Section~\ref{sec:exp:details}, we tune most hyperparameters of each baseline method by conducting a full grid search on the validation set of each dataset.
For other hyperparameters, we strictly follow the settings provided in their official code.
We train all models with the Adam ~\cite{kingma2014adam} optimizer with weight decay as $10^{-4}$, which is the same as in \method. 
The selected hyperparameter combination of each model is reported in Table~\ref{tab:HP_setting}.
The hyperparameter search space of baselines is as follows:
\begin{itemize}[leftmargin=*]
    \item \textbf{JODIE}: learning rate between ($10^{-3}$, $10^{-4}$), batch size among (200, 600, 1000)
    \item \textbf{DySAT}: learning rate between ($10^{-3}$, $10^{-4}$), batch size among (200, 600, 1000), and degree among (10, 100, 500)
    \item \textbf{TGAT}: learning rate between ($10^{-3}$, $10^{-4}$), batch size among (200, 600, 1000), and degree among (10, 100, 500)
    \item \textbf{TGN}: learning rate between ($10^{-3}$, $10^{-4}$), batch size among (200, 600, 1000), and degree among (10, 100, 500)
    \item \textbf{GraphMixer}: learning rate between ($10^{-3}$, $10^{-4}$), batch size among (200, 600, 1000), and degree among (10, 100, 500)
    \item \textbf{DyGFormer}: learning rate between ($10^{-3}$, $10^{-4}$), batch size among (200, 600, 1000), and maximum input sequence among (32, 64, 128)
    \item \textbf{JODIE+$\boldsymbol{RF}$}: learning rate between ($10^{-3}$, $10^{-4}$), batch size among (200, 600, 1000)
    \item \textbf{DySAT+$\boldsymbol{RF}$}: learning rate between ($10^{-3}$, $10^{-4}$), batch size among (200, 600, 1000), and degree among (10, 100, 500)
    \item \textbf{TGAT+$\boldsymbol{RF}$}: learning rate between ($10^{-3}$, $10^{-4}$), batch size among (200, 600, 1000), and degree among (10, 100, 500)
    \item \textbf{TGN+$\boldsymbol{RF}$}: learning rate between ($10^{-3}$, $10^{-4}$), batch size among (200, 600, 1000), and degree among (10, 100, 500)
    \item \textbf{GraphMixer+$\boldsymbol{RF}$}: learning rate between ($10^{-3}$, $10^{-4}$), batch size among (200, 600, 1000), and degree among (10, 100, 500)
    \item \textbf{DyGFormer+$\boldsymbol{RF}$}: learning rate between ($10^{-3}$, $10^{-4}$), batch size among (200, 600, 1000), and maximum input sequence among (32, 64, 128)
\end{itemize}
As we set a larger maximum node degree compared to previous studies, an out-of-memory (OOM) issue occurs when increasing the number of layers. 
Additionally, many studies~\cite{tgn_icml_grl2020,cong2022we} report that increasing the number of layers is ineffective.
Therefore, during tuning, we fix the number of layers to 1.

All baselines, like \method, first create dynamic node representations and then use a classifier to predict node properties. 
The classifier and the entire TGNN encoder are trained using label supervision.~\footnote{Previous studies explored pre-training the TGNN encoder using a link prediction task and freezing it while only training the classifier with label supervision. However, we found this approach less effective under significant distribution shifts, so we trained the TGNN encoder and the classifier together.}
TGNN baselines, except DyGFormer, are implemented using the TGL~\cite{zhou2022tgl} framework, while DyGFormer is implemented using the DyGLib~\cite{yu2023towards} framework. Since DyGFormer focuses on more sophisticated edge encoding, it generates the edge encoding and then extracts dynamic node representations. 
If no edge exists at the time of a node property query, the edge encoding from the most recent interaction before the query time is used.

\subsection{Detailed Hyperparameters of \method}
\label{sec:app:impl:model_param}
We train \method using the Adam optimizer, with a learning rate of $10^{-3}$ and a weight decay of $10^{-4}$. 
We fix the dropout probability to $0.2$.
In addition, we fix the scaling scalar of temporal encoding (Eq~\eqref{temporal_enc} in the main paper) to $\alpha = 10, \beta = 10$, and the dimension of a time encoding to 100.
We also set the dimension of the dynamic representation to 100, which is equivalent to the dimension of node features.
In the case of the weight of skip connection $\lambda_s$, we set 0 for the MOOC dataset and 1 for other datasets through validation.
In the positional node feature augmentation process, we utilize Node2Vec with walk length as 10, number of walks as 80, and return parameter p as 10 to generate node features for training nodes in the transductive approach.
We utilize the TGL~\cite{zhou2022tgl} framework for the implementation of \method.
