# Supplementary material for: Simple yet Effective Node Property Prediction on Edge Streams under Distribution Shifts
Source: arXiv:2504.00328 source file (2025-04-01)
Supplement: Supplementary file 6 [file 99_appendix_dataset_analysis.tex]

\section{APPENDIX: Real-world Dataset Analysis}
\label{sec:app:analysis}
