# Supplementary material for: Simple yet Effective Node Property Prediction on Edge Streams under Distribution Shifts
Source: arXiv:2504.00328 source file (2025-04-01)
Supplement: Supplementary file 7 [file 99_appendix_rebuttal_clean.tex]

%\input{tables/dataset}
%\input{tables/dataset}
\blue{
\section{Additional Experimental Results}
%\label{sec:app:dataset}
\subsection{Self-supervised Task with Edge Prediction}
\label{sec:app:SSL_edge}
In this subsection, we evaluate the performance of the link prediction-based self-supervised task. We train each neural network baseline method to perform edge prediction self-supervised task and use the target node's involved edge's prediction probability score as its anomaly score (without fine-tuning with labels). As shown in Table~\ref{tab:Edge_SSL_auc}, The edge prediction self-supervised task is less effective in performing dynamic anomaly detection compared to the node-wise self-supervised tasks (S1,S2) we proposed. In predicting the dynamic states of nodes, an edge-wise self-supervised task may result in a weaker expressive power to distinguish dynamic states compared to node-wise self-supervised tasks (S1, S2). Our additional edge frequency analysis in Fig~\ref{fig:Edge_SSL_analysis} supports this claim. 
If the edges that the anomalous state node is involved in are indeed unexpected, we would expect them to occur much less frequently compared to other normal edges in the dataset. Upon comparing the frequency distributions of normal edges and anomalous edges, we find that there is no clear distinction in the distributions.} %when detecting dynamic anomalies in edge streams.

\input{tables/rebuttal_edge_SSL_2}
%\vspace{-1cm}
\input{tables/rebutal_edge_SSL_analysis}
\blue{
\subsection{DTDG and Static Graph-based baselines}
In this subsection, We evaluate the dynamic anomaly detection performance of DTDG and static graph-based anomaly detection methods using real-world datasets. We utilize two SOTA DTDG-based approaches, StrGNN and TADDY (with a reduced number of epochs due to the long training time), and one static graph-based approach, DOMINANT. The experimental setting is the same as that of our Section 6.2 RQ1 experiment. 
We follow the hyperparameter settings provided by the existing DTDG papers with the exception of the number of epochs, which is reduced to 10 due to the long training time of DTDG methods.
Regarding DOMINANT, as there is no node feature in our datasets, we utilize identity vectors as node features.  
According to Table~\ref{tab:DTDG_static}, SLADE outperforms other baselines. We expect that this is because DTDG-based methods primarily aim for anomalous edge detection, which is less effective for (node-wise) dynamic anomaly detections, as mentioned in Section~\ref{sec:app:SSL_edge}, and the identity vector alone may not adequately represent attributed patterns in DOMINANT.}

\input{tables/rebuttal_DTDG_static}
\blue{
\subsection{Robustness to Anomalies in Training}
In this subsection, we assess SLADE's robustness to anomalies within the training set by comparing it with the baseline (SAD).
We augment the training dataset with increasing known abnormal edges, which are the edges involving nodes with the anomalous state in the training set, equivalent to X\% of the training dataset size, denoted as dataset+X\%. (These anomalies are treated as normal.)
The anomaly ratio in the Wikipedia test set is 0.186\%, while it is 0.09\% in the Reddit test set.
As shown in Table~\ref{tab:robust}, while the performance drop of SLADE is at most 0.023 AUROC, that of the baseline method is at most 0.691 AUROC. 
SLADE demonstrates good performance even in scenarios where abnormal data within the training dataset is significant (>10\% of total edge), showing its robustness.}

\input{tables/rebuttal_tolerance}

\blue{
\subsection{SLADE with Label Supervision}
In this subsection, we evaluate the variants of SLADE utilizing the proposed self-supervised tasks (S1, S2) as pretext tasks and fine-tuning them with labels.
We conduct additional experiments with fine-tuning and zero-shot settings. In this case, SLADE is first pre-trained with our proposed self-supervised tasks (S1, S2), and then dynamic representations (current memory, previous memory, generated memory) from SLADE and label information are utilized to fine-tune the MLP decoder (In the zero-shot setting, only normal labels are utilized). We define SLADE-FT as SLADE with fine-tuning and SLADE-ZS as SLADE with fine-tuning in a zero-shot setting.
As shown in Table~\ref{tab:fine_tuning}, surprisingly, our finding is that utilizing additional fine-tuning with label information is less effective than our method in most cases. 
We expect this is because our SSL task already aligns well with dynamic anomaly detection, while minimal anomaly label supervision may introduce issues such as distribution shift.
}

\input{tables/rebuttal_FT_ZS}
\blue{
\subsection{Large-scale Dataset}
We generated a large-scale synthetic dataset using the TGBL-coin dataset from the Temporal Graph Benchmark~\citep{huang2024temporal} Dataset. We reduce the dataset size (due to time constraints in the experiment) and preprocess the dataset by utilizing the same anomaly injection method in Section 6.2 RQ4, and it contains 499K nodes and 11M edges with a 1\% anomaly ratio.
Due to the significant resource and time requirements for training on such a large-scale dataset, we utilize only 30\% of the data for training and the remaining 70\% for testing.
For baselines, we employ rule-based methods and follow the same setting with RQ4 testing. 
We only modify the training epoch to 3 with fixed other hyperparameters in SLADE.
Our experimental result in Table~\ref{tab:large} demonstrates that SLADE also performs well on large-scale datasets compared to other baselines. Additionally, the average inference time per edge in the test set is $1.2 \times 10^{-4}$ seconds, which is aligned with the inference time per edge calculated in RQ2. This reaffirms that our method maintains constant inference time complexity regardless of graph size even in the large-scale dataset.}

\input{tables/rebuttal_large}
\blue{
\subsection{Learnable Time Encoding}
In this subsection, we evaluate the performance difference based on whether the time encoding is learned using the TGAT~\citep{xu2020inductive} approach or fixed using the GraphMixer~\citep{cong2022we} approach.
SLADE utilizes time encodings with fixed weights, as suggested by GraphMixer. We construct a variant of our model that utilizes learnable time encoding (SLADE-LT) from TGAT and compare it with SLADE with fixed time coding. According to Table~\ref{tab:TE}, we empirically verify that SLADE with fixed time encoding performs better. The reason for this might be fixing the weights of temporal encoding leads to a stable learning process, preventing the overfitting issue, as mentioned in GraphMixer.}

\input{tables/rebuttal_TE}
